# Supplementary material for: TRADE: Transducer-Augmented Decoder for Speech LLM
Source: arXiv:2606.08486 source file (2026-06-07)
Supplement: Supplementary file 1 [file appendix_training_loss.tex]

% ===============================================================
\section{Training Loss Curves: Blank-Rate Regularization Ablation}
\label{app:training_loss}

Figure~\ref{fig:training_loss} shows the training loss curves for the two configurations in our blank-rate regularization ablation (Section~\ref{sec:ablation}): the \textbf{baseline} ($\lambda=1.0$, with blank-rate regularization) and the \textbf{no-regularization} variant ($\lambda=0$), both trained on LibriSpeech-960h for 6{,}000 steps.

\begin{figure}[h]
\centering
\includegraphics[width=0.72\columnwidth]{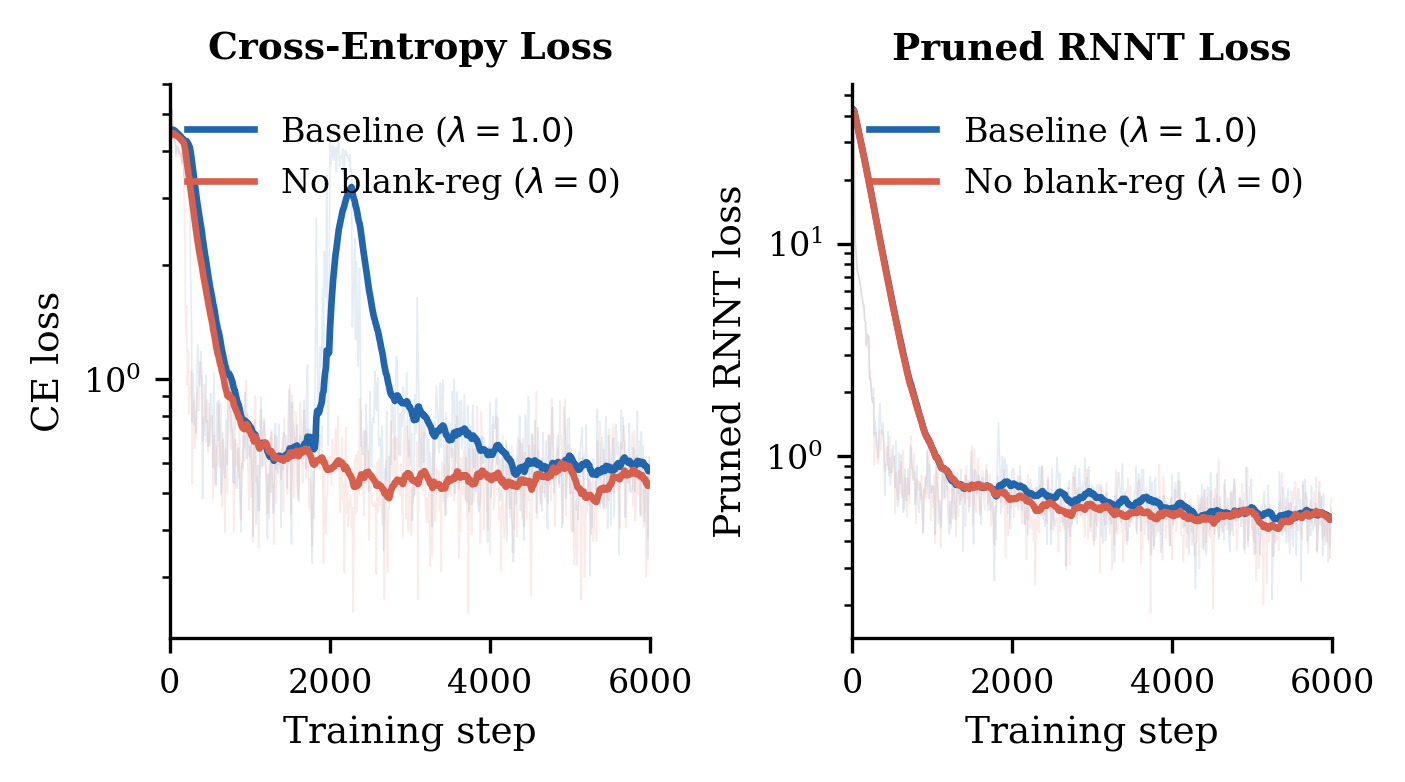}
\caption{Training loss curves for the baseline ($\lambda{=}1.0$, \textcolor[HTML]{2166AC}{blue}) and no-blank-reg ($\lambda{=}0$, \textcolor[HTML]{D6604D}{red}) configurations (log scale). Faint lines are raw per-step values; bold lines are exponential moving averages. \textbf{Left}: Cross-entropy loss. \textbf{Right}: Pruned RNNT loss.}
\label{fig:training_loss}
\end{figure}

Both configurations converge at similar rates in the early phase (steps 0--500).
Without blank-rate regularization, the CE loss drops faster and reaches a lower value earlier (steps $\approx$200--800), consistent with the model collapsing onto the LLM cross-entropy path via over-blanking.
The pruned RNNT loss is slightly higher for the baseline throughout training, as the blank-rate penalty prevents the transducer from ignoring acoustic frames and forces it to stay acoustically engaged.
